# Supplementary material for: Understanding Complexity in VideoQA via Visual Program Generation
Source: arXiv:2505.13429 source file (2025-05-19)
Supplement: Supplementary file 1 [file codegen_examples.tex]

\section{Code generation examples}
\label{sm:sec:additional_codegen}

We include additional results showing questions and their generated code. 
We group these into three sections corresponding to the three different complexity classes defined in Section \mainref{4.2} of the main paper: Single-Frame Easy in Table \ref{tab:single-frame-easy}, Single-Frame Complex in Table \ref{tab:single-frame-complex}, and Multi-Frame in Table \ref{tab:multi-frame}.
Additional questions, code and analysis can be found in the accompanying video.

%%%%%%%%%%%%%%%%%%%
% Single frame easy
\begin{table*}[ht]
\centering
\noindent\begin{tabular}{p{0.3\textwidth}|p{0.01\textwidth}p{0.69\textwidth}}
    \begin{minipage}[t]{0.3\textwidth}
        \textbf{Why is the boy in yellow reaching out to things on the green mat?} \\
        \centering
        \includegraphics[width=0.8\textwidth]{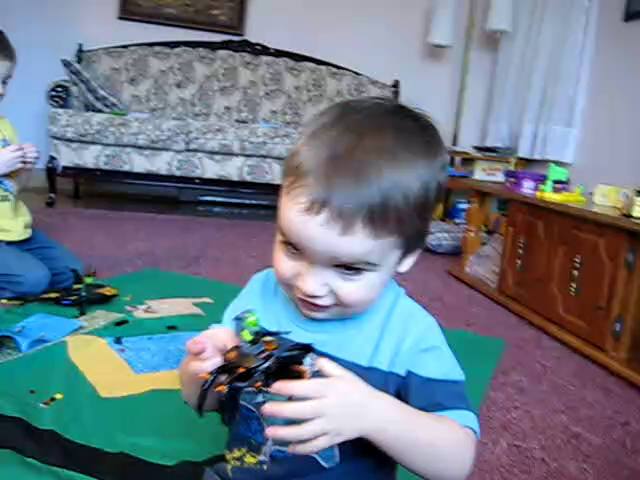} \\
    \end{minipage}
    & &
    \begin{minipage}[t]{0.65\textwidth}
        \inputcode{supplement/sample_codes/5.py}
    \end{minipage} \\
    \hline
    \begin{minipage}[t]{0.3\textwidth}
        \textbf{Why are there high chairs on the stage?} \\
        \centering
        \includegraphics[width=0.8\textwidth]{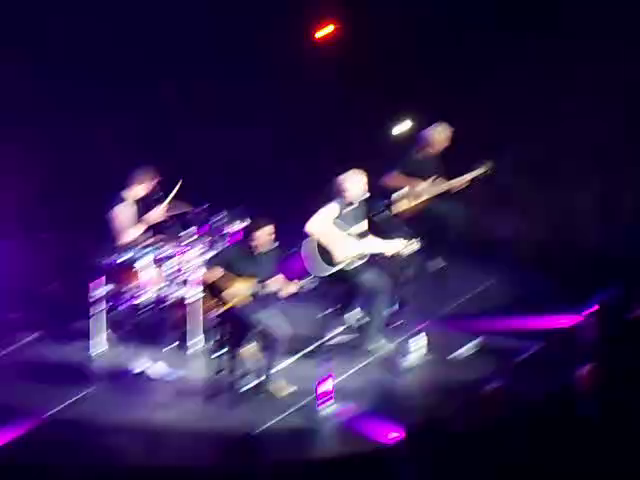} \\
    \end{minipage}
    & &
    \begin{minipage}[t]{0.65\textwidth}
        \inputcode{supplement/sample_codes/9.py}
    \end{minipage} \\
    \hline
    \begin{minipage}[t]{0.3\textwidth}
        \textbf{Where is this video taken?} \\
        \centering
        \includegraphics[width=0.8\textwidth]{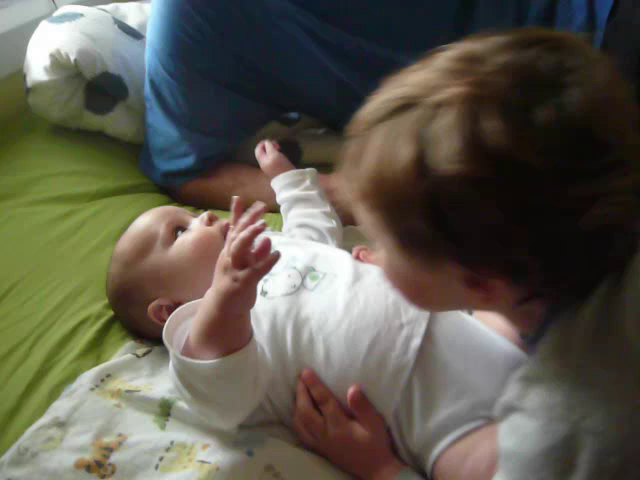} \\
    \end{minipage}
    & &
    \begin{minipage}[t]{0.65\textwidth}
        \inputcode{supplement/sample_codes/19.py}
    \end{minipage} \\
    \hline
\end{tabular}
\caption{Non cherry-picked Single Frame Easy Examples}
\label{tab:single-frame-easy}
\end{table*}

%%%%%%%%%%%%%%%%%%%
% Single frame hard
\begin{table*}[ht]
\centering
\noindent\begin{tabular}{p{0.3\textwidth}|p{0.01\textwidth}p{0.69\textwidth}}
    \begin{minipage}[t]{0.3\textwidth}
        \textbf{How do the two man play the instrument?} \\
        \centering
        \includegraphics[width=0.8\textwidth]{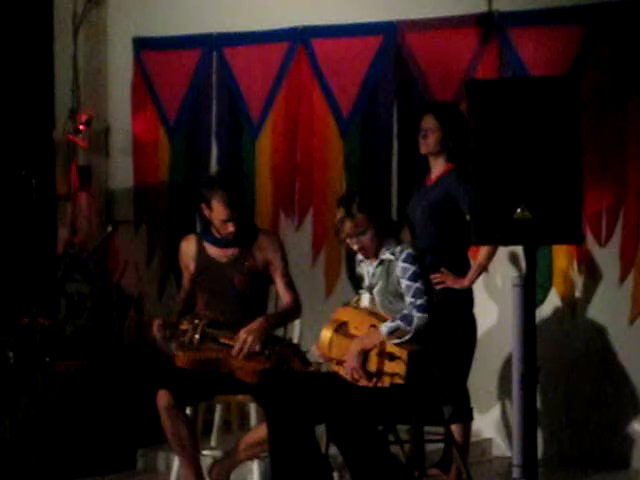} \\
    \end{minipage}
    & &
    \begin{minipage}[t]{0.65\textwidth}
        \inputcode{supplement/sample_codes/0.py}
    \end{minipage} \\
    \hline
    \begin{minipage}[t]{0.3\textwidth}
        \textbf{How does the man cycling try to sell the watch to the man in the trishaw?} \\
        \centering
        \includegraphics[width=0.8\textwidth]{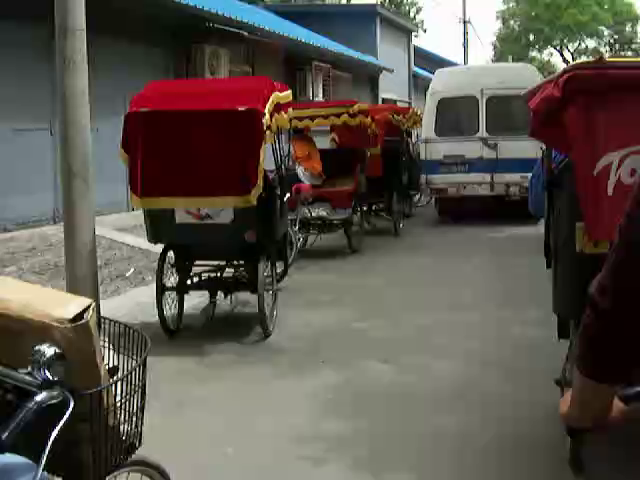} \\    \end{minipage}
    & &
    \begin{minipage}[t]{0.65\textwidth}
        \inputcode{supplement/sample_codes/2.py}
    \end{minipage} \\
    \hline
    \begin{minipage}[t]{0.3\textwidth}
        \textbf{Why did the man in white hold tightly to the boy in white?} \\
        \centering
        \includegraphics[width=0.8\textwidth]{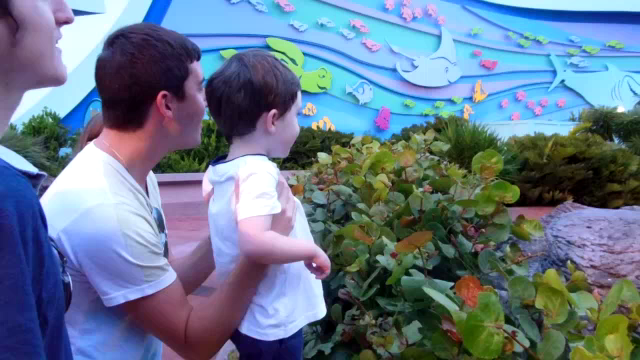} \\    \end{minipage}
    & &
    \begin{minipage}[t]{0.65\textwidth}
        \inputcode{supplement/sample_codes/4.py}
    \end{minipage} \\
    \hline
\end{tabular}
\caption{Non cherry-picked Single Frame Hard Examples}
\label{tab:single-frame-complex}
\end{table*}

%%%%%%%%%%%%%%%%%%%
% Multi-Frame Hard
\begin{table*}[ht]
\centering
\noindent\begin{tabular}{p{0.3\textwidth}|p{0.01\textwidth}p{0.69\textwidth}}
    \begin{minipage}[t]{0.3\textwidth}
        \textbf{What does the dog do after going to the cushion?} \\
        \centering
        \includegraphics[width=0.8\textwidth]{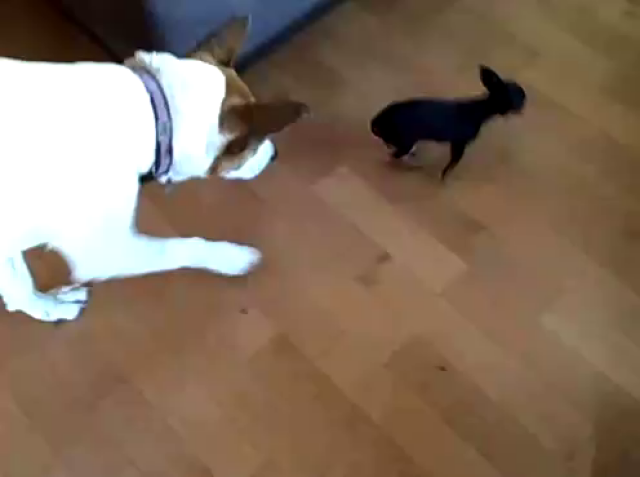} \\    \end{minipage}
    & &
    \begin{minipage}[t]{0.65\textwidth}
        \inputcode{supplement/sample_codes/3.py}
    \end{minipage} \\
    \hline
    \begin{minipage}[t]{0.3\textwidth}
        \textbf{How does the man in black feel after the dance?} \\
        \centering
        \includegraphics[width=0.8\textwidth]{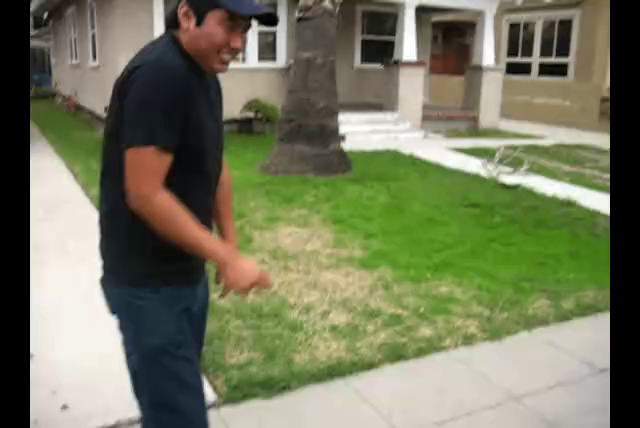} \\    \end{minipage}
    & &
    \begin{minipage}[t]{0.65\textwidth}
        \inputcode{supplement/sample_codes/87.py}
    \end{minipage} \\
    \hline
    % \begin{minipage}[t]{0.3\textwidth}
    %     \textbf{How did the man respond when he is stuck in the dirt?} \\
    %     \includegraphics[width=\textwidth]{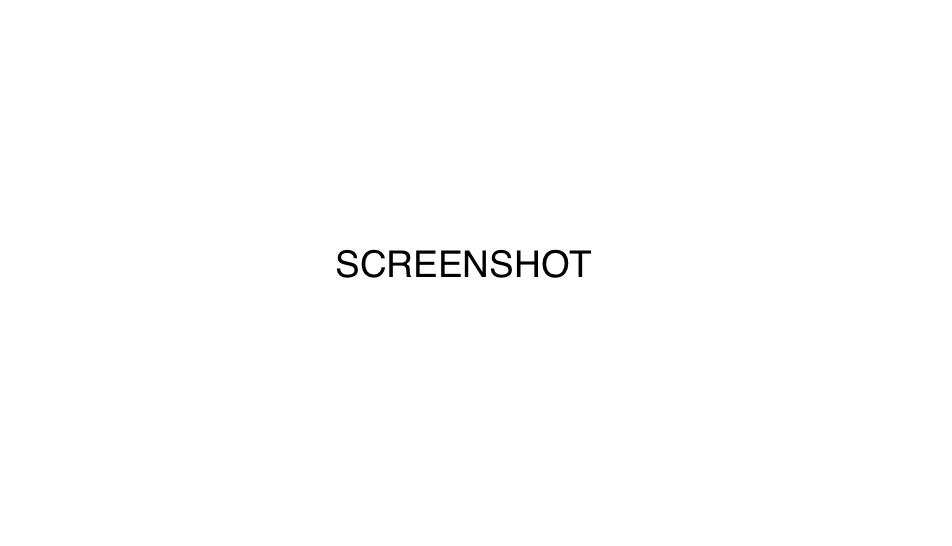} \\
    % \end{minipage}
    % & &
    % \begin{minipage}[t]{0.65\textwidth}
    %     \inputcode{supplement/sample_codes/16.py}
    % \end{minipage} \\
    % \hline
\end{tabular}
% \caption{Non cherry-picked Multi-Frame Hard Examples}
\end{table*}

\begin{table*}[ht]
\centering
\noindent\begin{tabular}{p{0.3\textwidth}|p{0.01\textwidth}p{0.69\textwidth}}
    \begin{minipage}[t]{0.3\textwidth}
        \textbf{How did the man respond when he is stuck in the dirt?} \\
        \centering
        \includegraphics[width=0.8\textwidth]{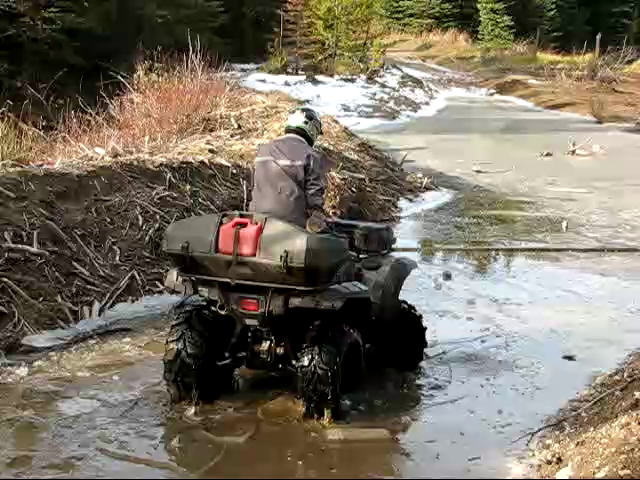} \\    \end{minipage}
    & &
    \begin{minipage}[t]{0.65\textwidth}
        \inputcode{supplement/sample_codes/16.py}
    \end{minipage} \\
    \hline
\end{tabular}
\caption{Non cherry-picked Multi-Frame Hard Examples}
\label{tab:multi-frame}
\end{table*}
